# Supplementary material for: Revealing hidden quantum correlations in an electromechanical measurement
Source: arXiv:1809.02396 ancillary file (2018-09-07)
Supplement: Supplementary file 1 [file ComplexSqueeze_Supplementary_material.pdf]

# Revealing hidden quantum correlations in an electromechanical measurement – Supplementary material

C. F. Ockeloen-Korppi,[1] E. Damskägg,[1] G. S. Paraoanu,[1] F. Massel,[2] and M. A. Sillanpää[1,*]

[1] *Department of Applied Physics, Aalto University, P.O. Box 15100, FI-00076 AALTO, Finland*
[2] *Department of Physics and Nanoscience Center, University of Jyväskylä, P.O. Box 35 (YFL), FI-40014 University of Jyväskylä, Finland*

## DERIVATION OF THE OUTPUT FIELD CORRELATORS

We derive here the equations of motion (EOMs) for the field and the mechanical quadratures generated by the linearized optomechanical Hamiltonian, extending the result given in [1] to finite pump detuning from the cavity resonance and to finite mismatch between the bichromatic sideband frequency $\omega_{\rm s}$ and the mechanical oscillator frequency $\omega_{\rm m}$. In a frame rotating at the pump frequency $\omega_{\rm p}$ the linearized Hamiltonian can be written as

$$H = \frac{\Delta}{2}\left(X^2 + Y^2\right) + 2GXQ \tag{S1}$$

where $\Delta = \omega_{\rm c} - \omega_{\rm p}$ and we have defined $X = (a^\dagger + a)/\sqrt{2}$, $Y = i(a^\dagger - a)\sqrt{2}$, $Q = (b^\dagger + b)/\sqrt{2}$, $P = i(b^\dagger - b)/\sqrt{2}$.

The quantum Langevin equations associated with the Hamiltonian given in Eq. (S1) can be written in the frequency domain as

$$\left(\frac{\kappa}{2} - i\omega\right) X = \Delta Y + \sqrt{\kappa} X_{\rm in} \tag{S2a}$$

$$\left(\frac{\kappa}{2} - i\omega\right) Y = -\Delta X - 2GQ + \sqrt{\kappa} Y_{\rm in} \tag{S2b}$$

$$\left(\frac{\gamma}{2} - i\omega\right) Q = \omega_{\rm m} P + \sqrt{\gamma} Q_{\rm in} \tag{S2c}$$

$$\left(\frac{\gamma}{2} - i\omega\right) P = -\omega_{\rm m} Q - 2GX + \sqrt{\gamma} P_{\rm in} \tag{S2d}$$

where all operators are evaluated at the frequency $\omega$, unless otherwise specified.

Solving Eqs. (S2a-S2d), we can express the relation between the input ($X_{\rm in}$, $Y_{\rm in}$) and the output ($X_{\rm o} = \sqrt{\kappa}X - X_{\rm in}$, $Y_{\rm o} = \sqrt{\kappa}Y - Y_{\rm in}$) quadratures for the cavity field as

$$X_{\rm o} = \mathcal{A}_{\rm XX} X_{\rm in} + \mathcal{A}_{\rm XY} Y_{\rm in} + \mathcal{A}_{\rm Xq} Q_{\rm in} + \mathcal{A}_{\rm Xp} P_{\rm in} \tag{S3a}$$

$$Y_{\rm o} = \mathcal{A}_{YX} X_{\rm in} + \mathcal{A}_{\rm YY} Y_{\rm in} + \mathcal{A}_{\rm Yq} Q_{\rm in} + \mathcal{A}_{\rm Yp} P_{\rm in} \tag{S3b}$$

where we have defined

$$\mathcal{A}_{\rm XX} = \kappa\eta\chi_{\rm c}\left(\frac{\kappa}{2} - i\omega\right) - 1, \qquad \mathcal{A}_{\rm XY} = \kappa\eta\chi_{\rm c}\Delta, \tag{S4a}$$

$$\mathcal{A}_{\rm YX} = -\kappa\eta\chi_{\rm c}\left(\Delta + 4G^2\omega_{\rm m}\chi_{\rm m}\right), \qquad \mathcal{A}_{\rm YY} = \kappa\eta\chi_{\rm c}\left(\frac{\kappa}{2} - i\omega\right) - 1, \tag{S4b}$$

$$\mathcal{A}_{\rm Xq} = -2\sqrt{\kappa\gamma}G\eta\chi_{\rm c}\chi_{\rm m}\Delta\left(\frac{\gamma}{2} - i\omega\right), \qquad \mathcal{A}_{\rm Xp} = -2\sqrt{\kappa\gamma}G\eta\chi_{\rm c}\chi_{\rm m}\Delta\omega_{\rm m}, \tag{S4c}$$

$$\mathcal{A}_{\rm Yq} = -2\sqrt{\kappa\gamma}G\eta\chi_{\rm c}\chi_{\rm m}\left(\frac{\kappa}{2} - i\omega\right)\left(\frac{\gamma}{2} - i\omega\right), \qquad \mathcal{A}_{\rm Yp} = -2\sqrt{\kappa\gamma}G\eta\chi_{\rm c}\chi_{\rm m}\left(\frac{\kappa}{2} - i\omega\right)\omega_{\rm m}. \tag{S4d}$$

with

$$\chi_{\rm c} = \left[\left(\frac{\kappa}{2} - i\omega\right)^2 + \Delta^2\right]^{-1}, \quad \chi_{\rm m} = \left[\left(\frac{\gamma}{2} - i\omega\right)^2 + \omega_{\rm m}^2\right]^{-1}, \quad \eta = \left[1 + 4G\omega_{\rm m}\chi_{\rm m}\Delta\chi_{\rm c}\right]^{-1}. \tag{S5}$$

From Eqs. (S3a, S3b), it is possible to evaluate the symmetrized covariance matrix for the output field correlator, which, owing to time translation invariance, becomes

$$C_{\rm i\,j}(\omega) = \frac{1}{2}\left\langle\left\{X_{\rm o}^{\rm i}(\omega), X_{\rm o}^{\rm j}(-\omega)\right\}\right\rangle \tag{S6}$$

where $\rm i, j = 1, 2$ ($X_{\rm o}^1 = X_{\rm o}$, $X_{\rm o}^2 = Y_{\rm o}$). Each element of $C_{\rm i\,j}(\omega)$ is written as the sum of a contribution originating from the mechanical thermal bath ($\langle\ldots\rangle_{\rm m}$) and a contribution associated with the cavity thermal bath ($\langle\ldots\rangle_{\rm c}$). Recognizing that, for each of the coefficients given in Eqs. (S4a-S4d) we have that $\mathcal{A}_{\rm ij}(-\omega) = \mathcal{A}_{\rm ij}^*(\omega)$, we can derive the following relations for the dependence of $C_{\rm i\,j}(\omega)$ on the bath field correlators

$$\frac{1}{2}\left\langle\left\{X_{\rm o}(\omega), X_{\rm o}(-\omega)\right\}\right\rangle_{\rm c} = \left[\left|\mathcal{A}_{\rm XX}\right|^2 + \left|\mathcal{A}_{\rm XY}\right|^2\right]\left(n_{\rm c} + \frac{1}{2}\right) \tag{S7a}$$

$$\frac{1}{2}\left\langle\left\{Y_{\rm o}(\omega), Y_{\rm o}(-\omega)\right\}\right\rangle_{\rm c} = \left[\left|\mathcal{A}_{\rm YX}\right|^2 + \left|\mathcal{A}_{\rm YY}\right|^2\right]\left(n_{\rm c} + \frac{1}{2}\right) \tag{S7b}$$

$$\frac{1}{2}\left\langle\left\{X_{\rm o}(\omega), Y_{\rm o}(-\omega)\right\}\right\rangle_{\rm c} = \left[\mathcal{A}_{\rm YX}\mathcal{A}_{\rm XX}{}^* + \mathcal{A}_{\rm YY}\mathcal{A}_{\rm XY}{}^*\right]\left(n_{\rm c} + \frac{1}{2}\right), \tag{S7c}$$

and on the mechanical field correlators

$$\frac{1}{2}\left\langle\left\{X_{\rm o}(\omega),X_{\rm o}(-\omega)\right\}\right\rangle_{\rm m}=\left[\left|\mathcal{A}_{\rm Xq}\right|^2+\left|\mathcal{A}_{\rm Xp}\right|^2\right]\left(n_{\rm m}+\frac{1}{2}\right) \tag{S8a}$$

$$\frac{1}{2}\left\langle\left\{Y_{\rm o}(\omega),Y_{\rm o}(-\omega)\right\}\right\rangle_{\rm m}=\left[\left|\mathcal{A}_{\rm Yq}\right|^2+\left|\mathcal{A}_{\rm Yp}\right|^2\right]\left(n_{\rm m}+\frac{1}{2}\right) \tag{S8b}$$

$$\frac{1}{2}\left\langle\left\{X_{\rm o}(\omega),Y_{\rm o}(-\omega)\right\}\right\rangle_{\rm m}=\left[\mathcal{A}_{\rm Yq}{\mathcal{A}_{\rm Xq}}^*+\mathcal{A}_{\rm Yp}{\mathcal{A}_{\rm Xp}}^*\right]\left(n_{\rm m}+\frac{1}{2}\right). \tag{S8c}$$

Eqs. (S7a, S7c) can be explicitly written as

$$\frac{1}{2}\left\langle\left\{X_{\rm o}(\omega),X_{\rm o}(-\omega)\right\}\right\rangle_{\rm c}=\kappa\left\{\kappa\left|\eta\right|^2\left|\chi_{\rm c}\right|^2\left(\frac{\kappa^2}{4}+\omega^2+\Delta^2\right)-2{\rm Re}\left[\eta\chi_{\rm c}\left(\frac{\kappa}{2}-i\omega\right)+1\right]\right\}\left(n_{\rm c}+\frac{1}{2}\right) \tag{S9a}$$

$$\begin{aligned}\frac{1}{2}\left\langle\left\{Y_{\rm o}(\omega),Y_{\rm o}(-\omega)\right\}\right\rangle_{\rm c}&=\kappa\left\{\kappa\left|\eta\right|^2\left|\chi_{\rm c}\right|^2\left(\frac{\kappa^2}{4}+\omega^2+\left|\Delta+4G^2\omega_{\rm m}\chi_{\rm m}\right|^2\right)\right.\\&\qquad\left.-2\,{\rm Re}\left[\eta\chi_{\rm c}\left(\frac{\kappa}{2}-i\omega\right)+1\right]\right\}\left(n_{\rm c}+\frac{1}{2}\right)\end{aligned} \tag{S9b}$$

$$\begin{aligned}\frac{1}{2}\left\langle\left\{X_{\rm o}(\omega),Y_{\rm o}(-\omega)\right\}\right\rangle_{\rm c}&=\kappa\left\{\kappa\left|\eta\right|^2\left|\chi_{\rm c}\right|^2\left[2\kappa G^2\omega_{\rm m}+2i\omega\left(\Delta+2G^2\omega_{\rm m}\chi_{\rm m}\right)\right]\right.\\&\qquad\left.+\eta\chi_{\rm c}\left(\Delta+4G^2\omega_{\rm m}\chi_{\rm m}\right)-\Delta\eta^*\chi_{\rm c}^*\right\}\left(n_{\rm c}+\frac{1}{2}\right)\end{aligned} \tag{S9c}$$

and Eqs. (S8a, S8c) become

$$\frac{1}{2}\left\langle\left\{X_{\rm o}(\omega),X_{\rm o}(-\omega)\right\}\right\rangle_{\rm m}=2\kappa\gamma\left|\eta\right|G^2\Delta^2\left|\chi_{\rm c}\right|^2\left|\chi_{\rm m}\right|^2\left(\gamma^2/4-\omega^2+\omega_{\rm m}^2\right)\left(n_{\rm m}+\frac{1}{2}\right) \tag{S10a}$$

$$\frac{1}{2}\left\langle\left\{Y_{\rm o}(\omega),Y_{\rm o}(-\omega)\right\}\right\rangle_{\rm m}=2\kappa\gamma\left|\eta\right|^2G^2\left(\kappa^2/4+\omega^2\right)\left|\chi_{\rm c}\right|^2\left|\chi_{\rm m}\right|^2\left(\gamma^2/4-\omega^2+\omega_{\rm m}^2\right)\left(n_{\rm m}+\frac{1}{2}\right) \tag{S10b}$$

$$\frac{1}{2}\left\langle\left\{X_{\rm o}(\omega),Y_{\rm o}(-\omega)\right\}\right\rangle_{\rm m}=2\kappa\gamma\left|\eta\right|G^2\Delta\,\kappa\left|\chi_{\rm c}\right|^2\left|\chi_{\rm m}\right|^2\left(\gamma^2/4-\omega^2+\omega_{\rm m}^2\right)\left(n_{\rm m}+\frac{1}{2}\right) \tag{S10c}$$

## COMPLEX DETECTION AND COVARIANCE MATRIX

In order to extract all information encoded in the covariance matrix, we consider the power spectrum resulting from the bichromatic detection:

$$S_{\rm bi}\left(\omega\right)=\frac{1}{2}\left\langle\left\{\Sigma(\omega),\Sigma(-\omega)\right\}\right\rangle \tag{S11}$$

where

$$\Sigma(\omega)=\frac{1}{\sqrt{2}}\left[\alpha_{\rm X}X_{\rm o}(\omega-\omega_s)+\alpha_{\rm X}^*X_{\rm o}(\omega+\omega_s)+\alpha_{\rm Y}Y_{\rm o}(\omega-\omega_s)+\alpha_{\rm Y}^*Y_{\rm o}(\omega+\omega_s)\right] \tag{S12}$$

where $\omega_{\rm s}$ is the detuning of the LO frequency from the pump tone. $S_{\rm bi}\left(\omega\right)$ can be written in terms of the covariance matrix $C_{\rm i\,j}(\omega)$ as

$$\begin{aligned}S_{\rm bi}(\omega)=&\frac{\left|\alpha_{\rm X}\right|^2}{2}\left[C_{1\,1}(\omega-\omega_{\rm s})+C_{1\,1}(\omega+\omega_{\rm s})\right]+\frac{\left|\alpha_{\rm Y}\right|^2}{2}\left[C_{2\,2}(\omega-\omega_{\rm s})+C_{2\,2}(\omega+\omega_{\rm s})\right]\\&+{\rm Re}\left[\alpha_{\rm A}\alpha_{\rm Y}C_{1\,2}\left(\omega-\omega_{\rm s}\right)+\alpha_{\rm X}^*\alpha_{\rm Y}^*C_{1\,2}\left(\omega+\omega_{\rm s}\right)\right]\end{aligned} \tag{S13}$$

which for $\omega=0$ and $\omega_{\rm s}=\omega_{\rm m}$, due to the frequency symmetry of $C_{\rm i\,j}(\omega)$, can be written as

$$\begin{aligned}S_{\rm bi}(0)=&\left|\alpha_{\rm X}\right|^2C_{1\,1}(\omega_{\rm s})+\left|\alpha_{\rm Y}\right|^2C_{2\,2}(\omega_{\rm s})\\&+2{\rm Re}\left[\alpha_{\rm X}\alpha_{\rm Y}C_{1\,2}\left(\omega_{\rm s}\right)\right]\end{aligned} \tag{S14}$$

The relation given by Eq. (S14) allows us to interpret $S_{\rm bi}(\omega)$ as a quadratic form associated with the matrix $C_{\rm i\,j}(\omega)$ in the variables $\alpha_{\rm X}$ and $\alpha_{\rm Y}$. Moreover, setting an arbitrary $\omega_{\rm s}$, the measurement $S_{\rm bi}(0)$ allows us to access the smallest (largest) eigenvalue of $C_{\rm i\,j}(\omega_{\rm s})$ by choosing $\alpha_{\rm X}$, $\alpha_{\rm Y}$ in such a way that the vector $(\alpha_{\rm X}, \alpha_{\rm Y})^{\rm T}$ correspond to the eigenvector associated to the smallest (largest) eigenvalue of $C_{\rm i\,j}(\omega_{\rm m})$, thus allowing us to access correlations hidden to homodyne detection. The special case $\omega_{\rm s} = \omega_{\rm m}$ essentially accesses the mechanical resonant frequency that shows the strongest noise reduction, and at the same time, the best sensitivity to external forces. Setting the two LO's exactly at the mechanical sidebands at either side of the pump tone is therefore the most relevant case. This case corresponds to the x-axis coordinate equal to zero in Fig. 5 in the main text.

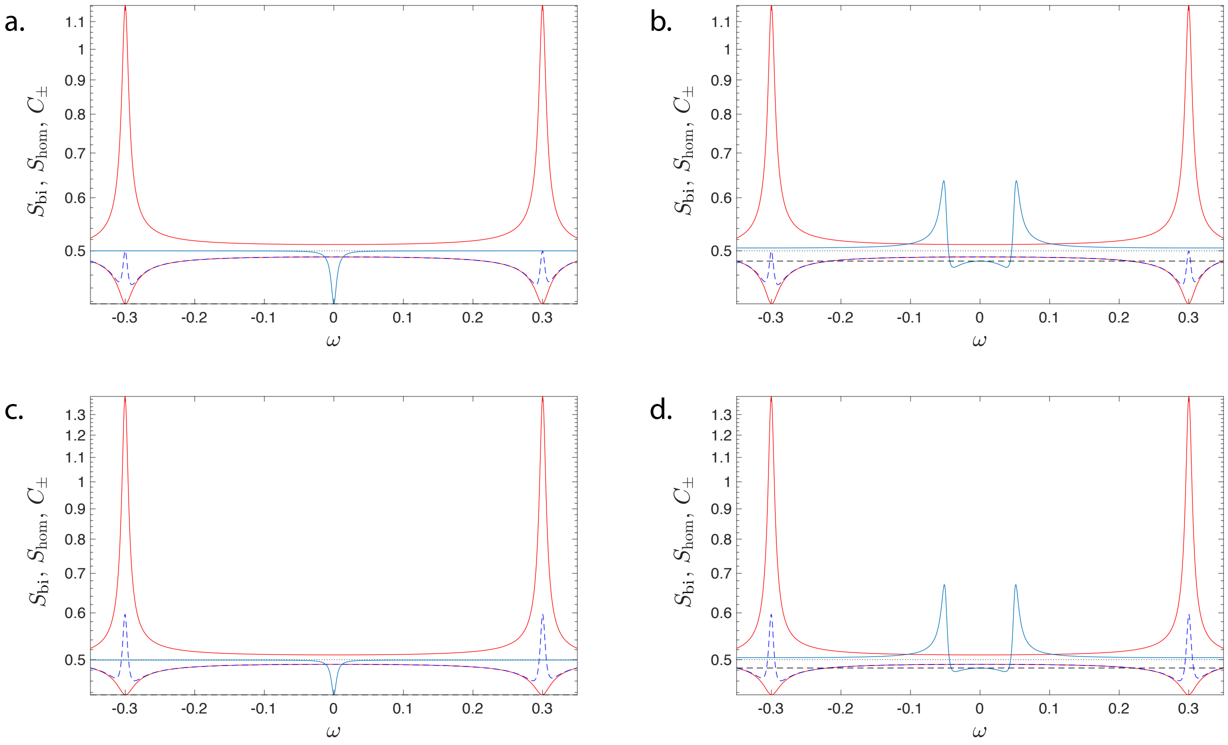


FIG. S1. Comparison between the bichromatic spectrum $S_{\rm bi}$ (blue line), the homodyne spectrum $S_{\rm hom}$ (blue dashed line) and the eigenvalues of $C_{\rm i,j}$ ($C_\pm$, red line) for $\omega_{\rm m}/\kappa = 0.3$. **a.** $\Delta = 0$, $\omega_{\rm s} = \omega_{\rm m}$; **b.** $\Delta = 0$, $\omega_{\rm s} = 1.003\,\omega_{\rm m}$; **c.** $\Delta/\kappa = -0.2$, $\omega_{\rm s} = \omega_{\rm m}$; **d.** $\Delta/\kappa = -0.2$, $\omega_{\rm s} = 1.003\,\omega_{\rm m}$.

In Fig. S1 we have compared the bichromatic and homodyne spectra $S_{\rm bi}$ and $S_{\rm hom}$ with the eigenvalues of $C_{\rm i,j}$ for $\Delta = 0$ and $\Delta/\kappa = 0.3$. We also consider the case $\omega_{\rm s} \neq \omega_{\rm m}$. From these plots it is possible to see how the frequency mismatch raises the value $S_{\rm bi}(0)$, while leaving the eigenvalues of $C_{\rm i,j}$ and the homodyne signal unaltered. Conversely, the choice $\Delta \neq 0$ affects the value of the homodyne signal at the mechanical resonance $\omega_{\rm m}$, increasing its value above the SQL. In the experiment, we chose a slightly red-detuned $\Delta$ in order to broaden the hidden window as compared to exact zero detuning, hence making it more clearly visible.

* mika.sillanpaa@aalto.fi

[1] L F Buchmann, S Schreppler, J Kohler, N Spethmann, and D M Stamper-Kurn, "Complex Squeezing and Force Measurement Beyond the Standard Quantum Limit," Phys. Rev. Lett. **117**, 030801–9 (2016).
